# Supplementary material for: Approximations of MINFLUX Localization Precision with Background
Source: arXiv:2410.12427 ancillary file (2025-01-08)
Supplement: Supplementary file 1 [file supplement.pdf]

# 1 D MINFLUX localization precision with background terms

The goal here is to understand the influence of background on MINFLUX precision. We follow the framework in Masullo et al. Biophys. Rep. 2022 (and in Yvan Eilers' thesis) to construct CRLB estimates for MINFLUX measurements using quadratic functions in 1D.

## Localization of emitters in 1D

### Minimum

For MINFLUX excitation, let's consider a quadratic equation

In[1]:=
```
f_quad[x_] := A * ((x0 - x) ^2 / σ_q^2 / 2) + A * b
```

The first order approximation of localization precision is

In[2]:=
```
dx_{0,quad} = FullSimplify[(1 / Sqrt[N] * f_quad[x] / D[f_quad[x], x0]) /. x → 0 /. b → 0]
```

Out[2]=

$$\frac{x0}{2\sqrt{N}}$$

### Minimum with known background

Now let's consider a quadratic measured at x=-L/2, L/2 in the case of a known background value.

In[3]:=
```
p0 = f_quad[-L / 2]; p1 = f_quad[L / 2]; psum = p0 + p1;
p0n = p0 / psum; p1n = p1 / psum;
σ_minK2sb = FullSimplify[
  Sqrt[1 / (N * (D[p0n, x0]^2 / p0n + D[p1n, x0]^2 / p1n))], {b > 0, N > 0, L > 0, σ_q > 0}]
```

Out[5]=

$$\frac{1}{4}\sqrt{\frac{\left(L^2+4\,x0^2+8\,b\,\sigma_q^2\right)^2\left(\left(L^2-4\,x0^2\right)^2+16\,b\,\sigma_q^2\left(L^2+4\,x0^2+4\,b\,\sigma_q^2\right)\right)}{L^2\,N\left(L^2-4\,x0^2+8\,b\,\sigma_q^2\right)^2}}$$

For b = 0, this simplifies to

In[6]:=
```
σ_minK2sbb0 = FullSimplify[σ_minK2sb /. b → 0, {L > 0, N > 0, x0 ∈ Reals}]
```

Out[6]=

$$\frac{L^2+4\,x0^2}{4\,L\,\sqrt{N}}$$

Which is equivalent to S22b in the Balzarotti 2017 paper supplement...

In[7]:=
```
FullSimplify[(L/(4 Sqrt[N]) (1 + (x0 / (L / 2))^2)) - σminK2sbb0, {N > 0, L > 0, x0 < L}]
```

Out[7]= 0

For x0 = 0 we obtain

In[8]:=
```
σminK2sbx0 = FullSimplify[σminK2sb /. x0 → 0, {L > 0, N > 0, b > 0, σq > 0}]
```

Out[8]=
$$\frac{L^2 + 8\, b\, \sigma_q^2}{4\, L\, \sqrt{N}}$$

And at x0=0, b=0, we get the standard equation (S22c in Balzarotti 2017)...

In[9]:=
```
σminK2sbb0x0 = FullSimplify[σminK2sbb0 /. x0 → 0, {L > 0, N > 0}]
```

Out[9]=
$$\frac{L}{4\, \sqrt{N}}$$

And if we evaluate the simple single-measurement first order approximation at $x_0 = L/2$, we obtain the same result:

In[10]:=
```
dx0,quad /. x0 → L / 2
```

Out[10]=
$$\frac{L}{4\, \sqrt{N}}$$

Now let’s consider a quadratic measured at x=-L/2, 0, L/2 in the case of a known background value.

In[11]:=
```
p0 = fquad[-L / 2]; p1 = fquad[L / 2]; p2 = fquad[0]; psum = p0 + p1 + p2;
p0n = p0 / psum; p1n = p1 / psum;
p2n = p2 / psum;
σminK3sb = FullSimplify[Sqrt[1 / (N * (D[p0n, x0]^2 / p0n +
        D[p1n, x0]^2 / p1n + D[p2n, x0]^2 / p2n))], {b > 0, N > 0, L > 0, σq > 0}]
```

Out[12]=
$$\frac{\sqrt{\frac{\left(x0^2+2\, b\, \sigma_q^2\right)\left(L^2+6\, x0^2+12\, b\, \sigma_q^2\right)^2\left(\left(L^2-4\, x0^2\right)^2+16\, b\, \sigma_q^2\left(L^2+4\, x0^2+4\, b\, \sigma_q^2\right)\right)}{L^2\, N\left(3\, x0^2\left(L^2-4\, x0^2\right)^2+4\, b\, \sigma_q^2\left(L^4+6\, L^2\, x0^2-24\, x0^4+4\, b\, \sigma_q^2\left(5\, L^2-12\, x0^2+24\, b\, \sigma_q^2\right)\right)\right)}}}{2\, \sqrt{2}}$$

For $x_0 = 0$, this simplifies to

In[13]:=
```
FullSimplify[σminK3sb /. x0 → 0, {σq > 0, N > 0, L > 0}]
```

Out[13]=
$$\frac{1}{4} \sqrt{\frac{\left(L^2 + 8\, b\, \sigma_q^2\right)\left(L^2 + 12\, b\, \sigma_q^2\right)}{L^2\, N}}$$

Because this is a case of known background, we can directly substitute values in the definition to compute the SBR at b=0.01:

In[14]:=
```
SBR_{x0=0} = psum / (3 * A * b) /. L → 50 /. σq → 250 /. x0 → 0 /. b → 0.01
```

Out[14]=
```
1.33333
```

## Minimum with unknown background

Now let's consider the K=3 case with unknown background.

In[15]:=
```
p0mat =
  {{D[p0n, x0]^2, D[p0n, x0] * D[p0n, b]}, {D[p0n, b] * D[p0n, x0], D[p0n, b]^2}};
p1mat =
  {{D[p1n, x0]^2, D[p1n, x0] * D[p1n, b]}, {D[p1n, b] * D[p1n, x0], D[p1n, b]^2}};
p2mat =
  {{D[p2n, x0]^2, D[p2n, x0] * D[p2n, b]}, {D[p2n, b] * D[p2n, x0], D[p2n, b]^2}};
J = FullSimplify[N * ((1 / p0n) * p0mat + (1 / p1n) * p1mat + (1 / p2n) * p2mat)];
invJ = FullSimplify[Inverse[J], {L > 0, A > 0, b > 0}];
σminK3 = FullSimplify[Sqrt[invJ[[1, 1]]]]
```

Out[20]=

$$\frac{1}{4}\sqrt{\frac{\left(L^2+6\,x0^2+12\,b\,\sigma_q^2\right)\left(L^4-12\,L^2\,x0^2+192\,x0^4+8\,b\left(L^2+48\,x0^2\right)\sigma_q^2\right)}{L^4\,N}}$$

Now let's make substitutions.

In[21]:=
```
σminK3s = FullSimplify[σminK3 /. x0 → xL * L /. b → bL * L * L / (σq * σq), {σq > 0, N > 0, L > 0}]
```

Out[21]=

$$\frac{1}{4}\,L\,\sqrt{\frac{\left(1+12\,b_L+6\,x_L^2\right)\left(1+8\,b_L+12\,(-1+32\,b_L)\,x_L^2+192\,x_L^4\right)}{N}}$$

For $x_0 = 0$ this simplifies to

In[22]:=
```
FullSimplify[σminK3 /. x0 → 0, {σq > 0, N > 0, L > 0}]
```

Out[22]=

$$\frac{1}{4}\sqrt{\frac{\left(L^2+8\,b\,\sigma_q^2\right)\left(L^2+12\,b\,\sigma_q^2\right)}{L^2\,N}}$$

which matches the known case.

Now let's plot a comparison of the unknown and known backgrounds.

In[23]:=
```
xx = {L → 50, σq → 250, b → 0.01, N → 100};
Plot[{σminK3sb /. xx, σminK3 /. xx}, {x0, 0, 25}, PlotStyle → {Blue, Red},
 PlotLegends → Placed[{"b known", "b unknown"}, {Left, Top}], PlotRange →
  {{0, 25}, {0, 20}}, FrameLabel → {{"σx0 (nm)", None}, {"x0 (nm)", None}}, Frame →
  {{True, False}, {True, False}}, LabelStyle → {FontSize → 14, FontFamily → "Arial"}]
```

Out[23]=

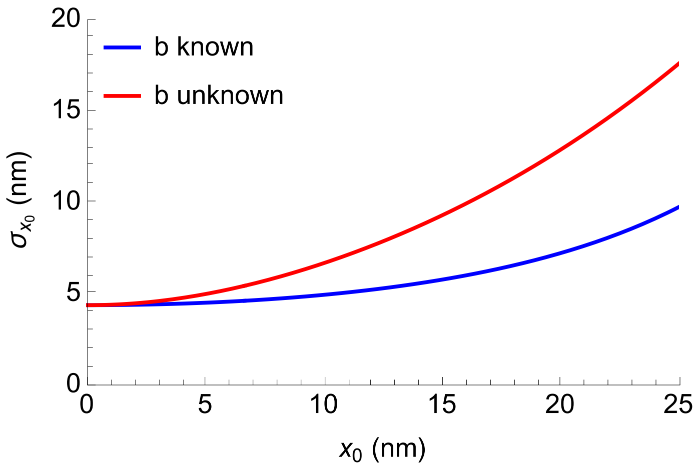


# Localization precision in the presence of different background sources

## K=2

Let’s consider the $x_0 = 0$ case. We can convert b and N to background photons Nb and signal photons Nb by making the observation that Nb=2Ab and $A = N_s / ((L/2 - x0)^2 / \sigma_q{}^2 / 2 + (L/2 + x0)^2 / \sigma_q{}^2 / 2)$.

In[24]:=
```
σminK2sbNsNb = FullSimplify[
  σminK2sb /. {b → (Nb * (((L / 2 - x0) ^2 / σq^2 / 2) + ((x0 - L / 2) ^2 / σq^2 / 2)) / (2 * Ns)),
     N → (Nb + Ns)} /. x0 → 0, {L > 0, Nb > 0, Ns > 0}]
```

Out[24]=

$$\frac{L \sqrt{N_b + N_s}}{4 N_s}$$

In the first instance, let’s consider the case where background comes from a non-perfect 0. In this case, Ntot = Ns.

In[25]:=
```
σminK2sbimperfect = FullSimplify[σminK2sb /. N → Ns /. x0 → 0, {L > 0, b > 0, σq > 0, Ns > 0}]
```

Out[25]=

$$\frac{L^2 + 8 b \sigma_q^2}{4 L \sqrt{N_s}}$$

Now let’s consider the case where background comes from out-of-focus fluorescence. In this case, we have to find the contribution from Ns and Nb.

In[26]:=
```
b_c = FullSimplify[
   (N_b * (((L / 2 - x0) ^2 / σ_q ^2 / 2) + ((x0 - L / 2) ^2 / σ_q ^2 / 2)) / (2 * N_s)) /. x0 → 0]
```
Out[26]=

$$\frac{L^2 N_b}{8 N_s \sigma_q^2}$$

Using this, we observe that Nb = 8 bNs$\sigma_q / L^2$ for the K=2 case. We substitute this back in to find

In[27]:=
```
σ_minK2sbbackground = FullSimplify[
   σ_minK2sb /. N → (N_b + N_s) /. x0 → 0 /. N_b → (8 * b * N_s * σ_q^2 / L^2), {L > 0, b > 0, σ_q > 0, N_s > 0}]
```
Out[27]=

$$\frac{1}{4}\sqrt{\frac{L^2 + 8\, b\, \sigma_q^2}{N_s}}$$

In[28]:=
```
Plot[{σ_minK2sbimperfect /. {b → 0.01, σ_q → 250, N_s → 100},
   σ_minK2sbbackground /. {b → 0.01, σ_q → 250, N_s → 100}},
  {L, 0, 200}, PlotStyle → {Blue, Red},
  PlotLegends → Placed[{"Imperfect zero", "Out-of-focus background"}, {Right, Top}],
  PlotRange → {{0, 200}, {0, 20}}, FrameLabel → {{"σ_x0 (nm)", None}, {"L (nm)", None}},
  Frame → {{True, False}, {True, False}},
  LabelStyle → {FontSize → 14, FontFamily → "Arial"}]
```
Out[28]=

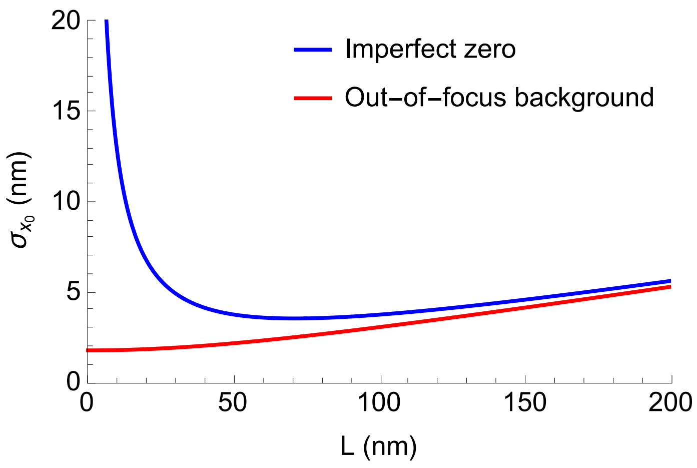


## K=3

Let's consider the $x_0 = 0$ case. We can convert b and N to background photons Nb and signal photons Nb by making the observation that Nb=3Ab and
$A = N_s / ((L/2 - x0)^2 / \sigma_q \char`^ 2/2 + (L/2 + x0)^2 / \sigma_q \char`^ 2/2 + x^2 / \sigma_q \char`^ 2/2)$.

In[29]:=
```
σminK3sbNsNb = FullSimplify[σminK3sb /.
    {b → (Nb * (((L / 2 - x0) ^ 2 / σq ^ 2 / 2) + ((x0 - L / 2) ^ 2 / σq ^ 2 / 2) + (x0 ^ 2 / σq ^ 2 / 2)) /
        (3 * Ns)), N → (Nb + Ns)} /. x0 → 0, {L > 0, Nb > 0, Ns > 0}]
```

Out[29]=

$$\frac{L \sqrt{\frac{2 N_b}{3} + N_s}}{4 N_s}$$

In the first instance, let’s consider the case where background comes from a non-perfect 0. In this case, Ntot = Ns.

In[30]:=
```
σminK3sbimperfect = FullSimplify[σminK3sb /. N → Ns /. x0 → 0, {L > 0, b > 0, σq > 0, Ns > 0}]
```

Out[30]=

$$\frac{\sqrt{\frac{\left(L^2+8 b \sigma_q^2\right) \left(L^2+12 b \sigma_q^2\right)}{N_s}}}{4 L}$$

Now let’s consider the case where background comes from out-of-focus fluorescence. In this case, we have to find the contribution from Ns and Nb.

In[31]:=
```
bc = FullSimplify[
  (Nb * (((L / 2 - x0) ^ 2 / σq ^ 2 / 2) + ((x0 - L / 2) ^ 2 / σq ^ 2 / 2) + (x0 ^ 2 / σq ^ 2 / 2)) /
     (3 * Ns)) /. x0 → 0]
```

Out[31]=

$$\frac{L^2 N_b}{12 N_s \sigma_q^2}$$

Using this, we observe that Nb = 12 bNs$\sigma_q / L^2$ for the K=3 case. We substitute this back in to find

In[32]:=
```
σminK3sbbackground =
 FullSimplify[σminK3sb /. N → (Nb + Ns) /. x0 → 0 /. Nb → (12 * b * Ns * σq^2 / L^2),
  {L > 0, b > 0, σq > 0, Ns > 0}]
```

Out[32]=

$$\frac{1}{4} \sqrt{\frac{L^2 + 8 b \sigma_q^2}{N_s}}$$

In[33]:=
```
Plot[{σminK3sbimperfect /. {b → 0.01, σq → 250, Ns → 100},
   σminK3sbbackground /. {b → 0.01, σq → 250, Ns → 100}},
  {L, 0, 200}, PlotStyle → {Blue, Red},
  PlotLegends → Placed[{"Imperfect zero", "Out-of-focus background"}, {Right, Top}],
  PlotRange → {{0, 200}, {0, 20}}, FrameLabel → {{"σx0 (nm)", None}, {"L (nm)", None}},
  Frame → {{True, False}, {True, False}},
  LabelStyle → {FontSize → 14, FontFamily → "Arial"}]
```

Out[33]=

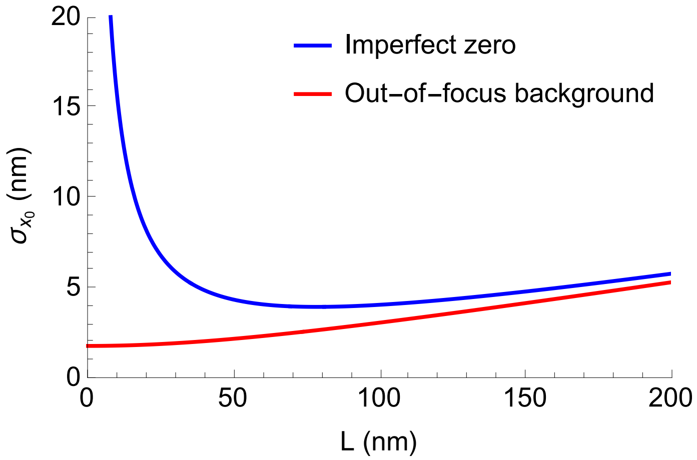


## Maximum

Suppose we use the Gaussian function to approximate the Airy maxima

In[34]:=
```
fGauss[x_] := A * Exp[- (x0 - x) ^2 / (2 * σq * σq)] + A * b
```

The first order approximation of the localization precision is

In[35]:=
```
dx0,Gauss = FullSimplify[(1 / Sqrt[N] * fGauss[x] / D[fGauss[x], x0]) /. x → 0 /. b → 0]
```

Out[35]=

$$-\frac{\sigma_q^2}{\sqrt{N}\ x0}$$

We can compare this to the minimum approximation:

In[36]:=
```
xx = {σq → 250, N → 100};
Plot[{dx0,quad /. xx, -dx0,Gauss /. xx}, {x0, 0, 250},
 PlotStyle → {Blue, Red}, PlotRange → {{0, 250}, {0, 175}},
 PlotLegends → Placed[{"Minimum", "Maximum"}, {Right, Top}],
 FrameLabel → {{"δx0 (nm)", None}, {"x0 (nm)", None}},
 Frame → {{True, False}, {True, False}},
 LabelStyle → {FontSize → 14, FontFamily → "Arial"}]
```

Out[37]=

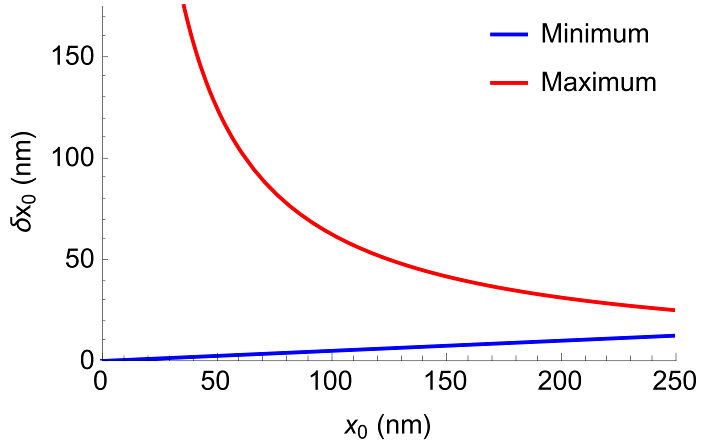


## Maximum with a known background

Let's consider the negative quadratic equation, an expansion of the 1D Gaussian.

In[38]:=
```
Series[A * Exp[- (x) ^2 / (2 * σq * σq)] + A * b, {x, 0, 2}]
```

Out[38]=

$$(A + A\,b) - \frac{A\,x^2}{2\,\sigma_q^2} + O[x]^3$$

In[39]:=
```
fnegquad[x_] := A * (1 - ((x0 - x) / σq) ^2 / 2) + A * b
p0 = fnegquad[-L / 2]; p1 = fnegquad[L / 2]; psum = p0 + p1;
p0n = p0 / psum; p1n = p1 / psum;
σmaxK2sb = FullSimplify[
  Sqrt[1 / (N * (D[p0n, x0]^2 / p0n + D[p1n, x0]^2 / p1n))], {b > 0, N > 0, L > 0, σq > 0}]
```

Out[42]=

$$\frac{1}{4}\sqrt{\frac{\left(L^2 + 4\,x0^2 - 8\,(1+b)\,\sigma_q^2\right)^2 \left(\left(L^2 - 4\,x0^2\right)^2 - 16\,(1+b)\,\left(L^2 + 4\,x0^2\right)\sigma_q^2 + 64\,(1+b)^2\,\sigma_q^4\right)}{L^2\,N\,\left(L^2 - 4\,x0^2 - 8\,(1+b)\,\sigma_q^2\right)^2}}$$

For x0=0 this simplifies to

In[43]:=
```
FullSimplify[σmaxK2sb /. x0 → 0, {σq > 0, N > 0, L > 0, bL > 0}]
```
Out[43]=

$$\frac{1}{4}\sqrt{\frac{\left(L^2-8\,(1+b)\,\sigma_q^2\right)^2}{L^2\,N}}$$

For x0=0 and no background we get:

In[44]:=
```
FullSimplify[σmaxK2sb /. x0 → 0 /. b → 0, {σq > 0, N > 0, L > 0}]
```
Out[44]=

$$\frac{\mathrm{Abs}\left[L^2-8\,\sigma_q^2\right]}{4\,L\,\sqrt{N}}$$

Now let’s consider the Gaussian case.

In[45]:=
```
p0 = fGauss[-L / 2]; p1 = fGauss[L / 2]; psum = p0 + p1;
p0n = p0 / psum; p1n = p1 / psum;
σGK2sb = FullSimplify[
  Sqrt[1 / (N * (D[p0n, x0]^2 / p0n + D[p1n, x0]^2 / p1n))], {b > 0, N > 0, L > 0, σq > 0}]
```
Out[47]=

$$2\sqrt{\frac{e^{-\frac{L^2+4\,x0^2}{4\,\sigma_q^2}}\left(1+b\,e^{\frac{(L-2\,x0)^2}{8\,\sigma_q^2}}\right)\left(1+b\,e^{\frac{(L+2\,x0)^2}{8\,\sigma_q^2}}\right)\left(e^{\frac{(L-2\,x0)^2}{8\,\sigma_q^2}}+e^{\frac{(L+2\,x0)^2}{8\,\sigma_q^2}}+2\,b\,e^{\frac{L^2+4\,x0^2}{4\,\sigma_q^2}}\right)^2\sigma_q^4}{N\left(2\,L+b\,e^{\frac{(L-2\,x0)^2}{8\,\sigma_q^2}}\,L+b\,e^{\frac{(L+2\,x0)^2}{8\,\sigma_q^2}}\,(L-2\,x0)+2\,b\,e^{\frac{(L-2\,x0)^2}{8\,\sigma_q^2}}\,x0\right)^2}}$$

At x0=0, this becomes

In[48]:=
```
FullSimplify[σGK2sb /. x0 → 0, {L > 0, N > 0, σq > 0, b > 0}]
```
Out[48]=

$$\frac{2\left(1+b\,e^{\frac{L^2}{8\,\sigma_q^2}}\right)\sigma_q^2}{L\,\sqrt{N}}$$

Let’s plot this as a function of b and L.

In[49]:=
```
xx = {x0 → 0, σq → 250, N → 100};
Plot[{σGK2sb /. xx /. b → 0, σGK2sb /. xx /. b → 0.01, σGK2sb /. xx /. b → 0.1},
 {L, 0, 2000}, PlotRange → {{0, 2000}, {0, 175}}, PlotStyle → {Blue, Red, Cyan},
 PlotLegends → Placed[{"b=0", "b=0.01", "b=0.1"}, {Center, Top}],
 FrameLabel → {{"σx0(x0=0)  (nm)", None}, {"L  (nm)", None}},
 Frame → {{True, False}, {True, False}},
 LabelStyle → {FontSize → 14, FontFamily → "Arial"}]
```

Out[50]=

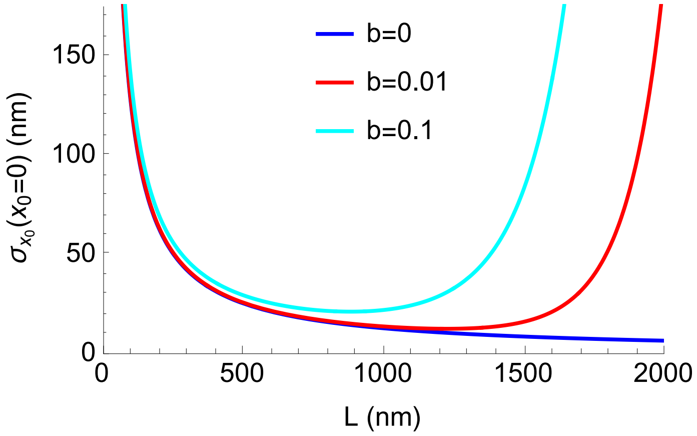


At b = 0, this becomes

In[51]:=
```
σGK2sbb0 = FullSimplify[σGK2sb /. b → 0, {L > 0, N > 0, σq > 0, x0 < L}]
```

Out[51]=

$$\frac{2\,\mathrm{Cosh}\left[\frac{L\,x0}{2\,\sigma_q^2}\right]\sigma_q^2}{L\,\sqrt{N}}$$

This is equivalent to S23b in Balzarotti 2017 in the event you swap his definition of a Gaussian with ours...namely 4*Log[2] becomes (1/2)...

In[52]:=
```
FullSimplify[σGK2sbb0 - (1 / Sqrt[N] * σq^2 / L * 2 * Cosh[x0 * L / (2 * σq^2)]),
 {L > 0, N > 0, σq > 0, x0 < L}]
```

Out[52]=

0

And at x0=0, b=0, this is again in agreement with S24b in Balzarotti 2017 if you swap 1/(4*Log[2]) for 2...

In[53]:=
```
FullSimplify[σGK2sb /. x0 → 0 /. b → 0, {L > 0, N > 0, σq > 0, x0 < L}]
```

Out[53]=

$$\frac{2\,\sigma_q^2}{L\,\sqrt{N}}$$

This is the same as the simple single measurement approximation evaluated at -L/2

In[54]:=
```
dx0,Gauss /. x0 → -L / 2
```
Out[54]=

$$\frac{2\,\sigma_q^2}{L\,\sqrt{N}}$$

## Comparison of minima and maxima

First, let’s do a quick comparison of the K=2 cases for the maximums and minimum evaluated in the presence of background.

In[55]:=
```
xx = {σq → 250, x0 → 0, N → 100, b → 0.01};
pl0 = Plot[{σminK2sb /. xx, σGK2sb /. xx, σmaxK2sb /. xx}, {L, 0, 250}, PlotStyle → {Blue,
    Red, {Red, Dashed}}, PlotLegends → Placed[{"Minimum", "Maximum, Gaussian",
     "Maximum, quadratic"}, {Right, Top}], FrameLabel → {{"σx0 (x0=0)  (nm)", None},
    {"L  (nm)", None}}, Frame → {{True, False}, {True, False}}, PlotRange →
   {{0, 250}, {0, 175}}, LabelStyle → {FontSize → 14, FontFamily → "Arial"}]
pl1 = Plot[{σminK2sb /. xx, σGK2sb /. xx}, {L, 0, 1000},
  PlotStyle → {Blue, Red}, LabelStyle → {FontSize → 14, FontFamily → "Arial"}]
Show[pl0, pl1]
```
Out[55]=

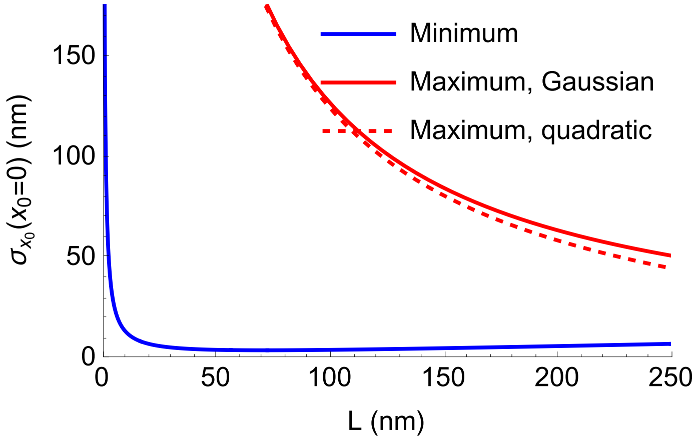


Out[56]=

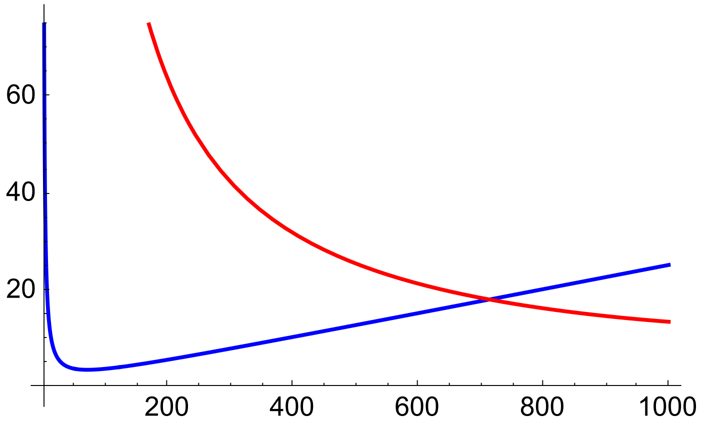

Out[57]=

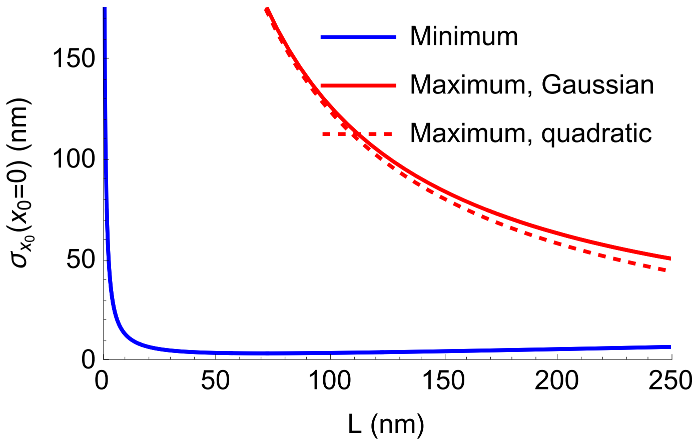


Now, let's do the main text figures.

In[58]:=
```
xx = {σq → 250, x0 → 0, N → 100};
Plot[{σminK2sb /. xx /. b → 0, σGK2sb /. xx /. b → 0}, {L, 0, 250}, PlotStyle → {Blue, Red},
 PlotLegends → Placed[{"Minimum, b=0", "Maximum"}, {Right, Top}],
 FrameLabel → {{"σx0 (x0=0) (nm)", None}, {"L (nm)", None}},
 Frame → {{True, False}, {True, False}}, PlotRange → {{0, 250}, {0, 175}},
 LabelStyle → {FontSize → 18, FontFamily → "Helvetica"}]
```

Out[59]=

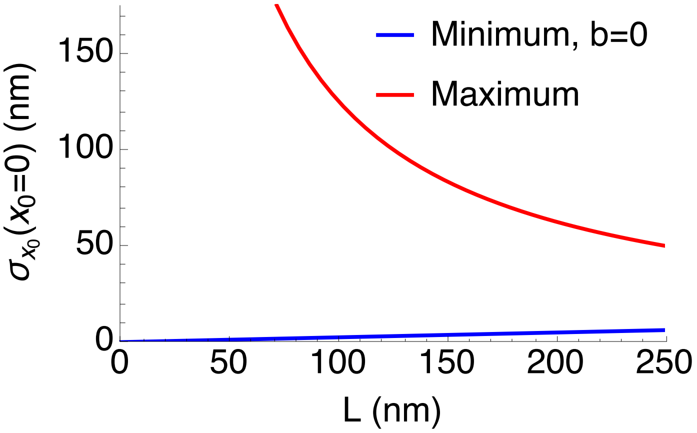

In[60]:=
```
Plot[{σminK2sb /. xx /. b → 0, σminK2sb /. xx /. b → 0.01, σminK2sb /. xx /. b → 0.1},
 {L, 0, 250}, PlotStyle → {Blue, {Blue, Dashed}, {Blue, Dotted}},
 PlotLegends → Placed[{"b=0", "b=0.01", "b=0.1"}, {Right, Top}],
 FrameLabel → {{"σx0(x0=0) (nm)", None}, {"L (nm)", None}},
 Frame → {{True, False}, {True, False}}, PlotRange → {{0, 100}, {0, 35}},
 LabelStyle → {FontSize → 18, FontFamily → "Helvetica"}]
```

Out[60]=

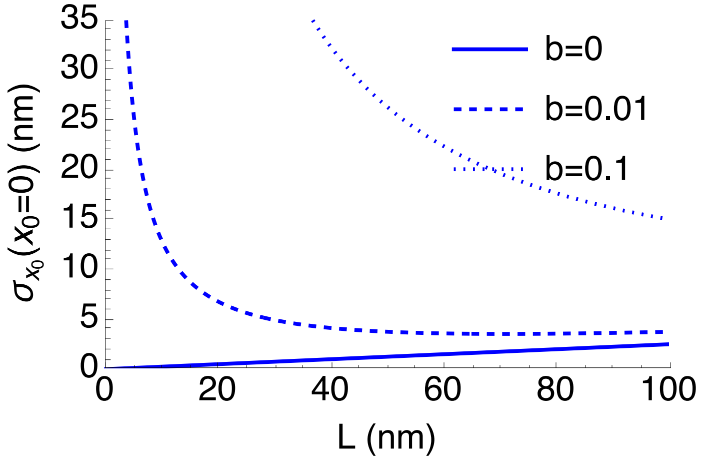


# Localization of emitters in 2D

## First, a 1D donut for sanity

In[61]:= $f[x\_, s\_] := A * 4 * Exp[1] * Log[2] * \frac{(x - x0)^2}{s^2} * Exp\left[-4 * Log[2] * \frac{(x - x0)^2}{s^2}\right]$

In[62]:=
```
p0 = f[-L / 2, σq];
p1 = f[L / 2, σq];
psum = p0 + p1;
p0n = p0 / psum;
p1n = p1 / psum;
```

In[67]:= $\sigma_{donut1D} = Sqrt\left[1 / \left(N * \left(D[p0n, x0]^2 / p0n + D[p1n, x0]^2 / p1n\right)\right)\right];$

In[68]:= FullSimplify[$\sigma_{donut1D}$ /. x0 → 0, {L > 0, $\sigma_q$ > 0, $\sigma_q$ > L, N > 0}]

Out[68]=

$$\frac{L}{\sqrt{N}\left(4 - \frac{4 L^2 Log[2]}{\sigma_q^2}\right)}$$

OK, this matches equation S22f in the Balzarotti 2017 supplement.

## 2D MINFLUX with known background

In[69]:=
```
ang2x[tx_, R_] := R * Cos[tx]
ang2y[ty_, R_] := R * Sin[ty]
R = L / 2;
```

Let’s construct a donut following the definition in Eilers Section 2.1, but add a background term.

In[72]:=
```
f[x_, y_, s_] :=
  A * 4 * Exp[1] * Log[2] * ((x - x0)^2 + (y - y0)^2)/s^2 * Exp[-4 * Log[2] * ((x - x0)^2 + (y - y0)^2)/s^2] + A * b
```

In[73]:=
```
p0 = f[0, 0, σq] // Simplify;
p1 = f[ang2x[2 π / 3, R], ang2y[2 π / 3, R], σq] // Simplify;
p2 = f[ang2x[4 π / 3, R], ang2y[4 π / 3, R], σq] // Simplify;
p3 = f[ang2x[2 π, R], ang2y[2 π, R], σq] // Simplify;
psum = (p0 + p1 + p2 + p3) // Simplify;
p0n = (p0 / psum) // Simplify;
p1n = (p1 / psum) // Simplify;
p2n = (p2 / psum) // Simplify;
p3n = (p3 / psum) // Simplify;
p0mat =
  {{D[p0n, x0] ^ 2, D[p0n, x0] * D[p0n, y0]}, {D[p0n, y0] * D[p0n, x0], D[p0n, y0] ^ 2}};
p1mat =
  {{D[p1n, x0] ^ 2, D[p1n, x0] * D[p1n, y0]}, {D[p1n, y0] * D[p1n, x0], D[p1n, y0] ^ 2}};
p2mat =
  {{D[p2n, x0] ^ 2, D[p2n, x0] * D[p2n, y0]}, {D[p2n, y0] * D[p2n, x0], D[p2n, y0] ^ 2}};
p3mat =
  {{D[p3n, x0] ^ 2, D[p3n, x0] * D[p3n, y0]}, {D[p3n, y0] * D[p3n, x0], D[p3n, y0] ^ 2}};
J = N * ((1 / p0n) * p0mat + (1 / p1n) * p1mat + (1 / p2n) * p2mat + (1 / p3n) * p3mat);
invJ = Assuming[{L > 0, σq > 0, σq > L, N > 0, A > 0, x0 > 0, y0 > 0, b > 0},
   Inverse[J /. x0 → 0 /. y0 → 0]];
σMF = Sqrt[Tr[invJ / 2]];
```

And compute the localization precision

In[85]:=
```
σMFr0 = FullSimplify[σMF /. {x0 → 0, y0 → 0, b → 0}, {L > 0, σq > 0, σq > L, N > 0, A > 0}]
```

Out[85]=

$$\frac{L\,\sigma_q^2}{\sqrt{2}\,\sqrt{N}\,\left(-L^2\,\mathrm{Log}[4]+2\,\sigma_q^2\right)}$$

Let’s confirm this matches Balzarotti S27...

In[86]:=

$$\texttt{FullSimplify}\left[\sigma_{\texttt{MFr0}} - \frac{\texttt{L}}{\texttt{2 * Sqrt[2 * N]}} \Big/ \left(1 - \frac{\texttt{L}^2 \texttt{ * Log[2]}}{\sigma_q{}^2}\right)\right]$$

Out[86]=

```
0
```

...hooray!

Now let's check the equivalence to Balzarotti 2017 S31, which is computed with SBR...

In[87]:=

$$\sigma_{\texttt{MFr0b}} = \texttt{FullSimplify}[\sigma_{\texttt{MF}} \texttt{ /. x0} \to \texttt{0 /. y0} \to \texttt{0, \{L > 0, } \sigma_q \texttt{ > 0, } \sigma_q \texttt{ > L, N > 0, A > 0\}]}$$

Out[87]=

$$\frac{\sqrt{\dfrac{\sigma_q^4 \left(e\, L^2 \,\text{Log}[8] + 2^{2+\frac{L^2}{\sigma_q^2}}\, b\, \sigma_q^2\right)\left(e\, L^2 \,\text{Log}[2] + 2^{\frac{L^2}{\sigma_q^2}}\, b\, \sigma_q^2\right)}{N \left(L^3 \,\text{Log}[2] - L\, \sigma_q^2\right)^2}}}{\sqrt{6}\; e\; \text{Log}[4]}$$

Let's consider the $x_0 = 0$, $y_0 = 0$ case. Applying the definition of SBR in the K=4 case, we see that b = $\Sigma_i f_{\text{nobg}}(-x_i)/(4*A*\text{sbr})$...

In[88]:=

$$\sigma_{\texttt{MFr0sbr}} = \texttt{FullSimplify}[\sigma_{\texttt{MFr0b}} \texttt{ /. b} \to \texttt{(psum - 4 * A * b) / (4 * A * sbr) /. x0} \to \texttt{0 /. y0} \to \texttt{0,}$$
$$\texttt{\{L > 0, } \sigma_q \texttt{ > 0, } \sigma_q \texttt{ > L, N > 0, A > 0, sbr > 0\}]}$$

Out[88]=

$$\frac{L \sqrt{\dfrac{(1+\text{sbr})\ (3+4\,\text{sbr})}{N}}\ \sigma_q^2}{4\,\sqrt{2}\ \text{sbr}\ \left(-L^2 \,\text{Log}[2] + \sigma_q^2\right)}$$

In[89]:=

$$\texttt{FullSimplify}\Bigg[$$
$$\sigma_{\texttt{MFr0sbr}} - \left(\frac{\texttt{L}}{\texttt{2 * Sqrt[2 * N]}} \Big/ \left(1 - \frac{\texttt{L}^2 \texttt{ * Log[2]}}{\sigma_q{}^2}\right)\right) \texttt{ * Sqrt[(1 + 1 / sbr) * (1 + 3 / (4 * sbr))],}$$
$$\texttt{\{L > 0, } \sigma_q \texttt{ > 0, } \sigma_q \texttt{ > L, N > 0, A > 0, sbr > 0\}}\Bigg]$$

Out[89]=

```
0
```

And we see this indeed matches S31 with a change of variables.

## Orbital tracking

Let's try constructing orbital tracking measured at only three evenly distributed points on a circle.

In[90]:=
```
f[x_, y_, s_] := A * Exp[-(x - x0)^2 / (2 * s * s)] * Exp[-(y - y0)^2 / (2 * s * s)] + A * b
p0 = f[ang2x[0, R], ang2y[0, R], σq]; p1 = f[ang2x[2 π / 3, R], ang2y[2 π / 3, R], σq];
p2 = f[ang2x[4 π / 3, R], ang2y[4 π / 3, R], σq]; psum = p0 + p1 + p2;
p0n = p0 / psum; p1n = p1 / psum; p2n = p2 / psum;
p0mat =
  {{D[p0n, x0]^2, D[p0n, x0] * D[p0n, y0]}, {D[p0n, y0] * D[p0n, x0], D[p0n, y0]^2}};
p1mat =
  {{D[p1n, x0]^2, D[p1n, x0] * D[p1n, y0]}, {D[p1n, y0] * D[p1n, x0], D[p1n, y0]^2}};
p2mat =
  {{D[p2n, x0]^2, D[p2n, x0] * D[p2n, y0]}, {D[p2n, y0] * D[p2n, x0], D[p2n, y0]^2}};
J = N * ((1 / p0n) * p0mat + (1 / p1n) * p1mat + (1 / p2n) * p2mat);
invJ = Inverse[J];
σOT = Sqrt[Tr[invJ] / 2];
```

In[99]:=
```
σOTx0 = FullSimplify[σOT /. x0 → 0 /. y0 → 0, {σq > 0, N > 0, L > 0, b > 0}]
```

Out[99]=

$$\frac{2\sqrt{2}\left(1 + b\, e^{\frac{L^2}{8\sigma_q^2}}\right)\sigma_q^2}{L\sqrt{N}}$$

Let's plot this as a function of L and b.

In[100]:=
```
xx = {x0 → 0, y0 → 0, σq → 250, N → 100};
Plot[{σOT /. xx /. b → 0, σOT /. xx /. b → 0.01, σOT /. xx /. b → 0.1},
 {L, 0, 2000}, PlotRange → {{0, 2000}, {0, 175}}, PlotStyle → {Blue, Red, Cyan},
 PlotLegends → Placed[{"b=0", "b=0.01", "b=0.1"}, {Center, Top}],
 FrameLabel → {{"σx₀(x₀=0,y₀=0) (nm)", None}, {"L (nm)", None}},
 Frame → {{True, False}, {True, False}},
 LabelStyle → {FontSize → 14, FontFamily → "Arial"}]
```

Out[101]=

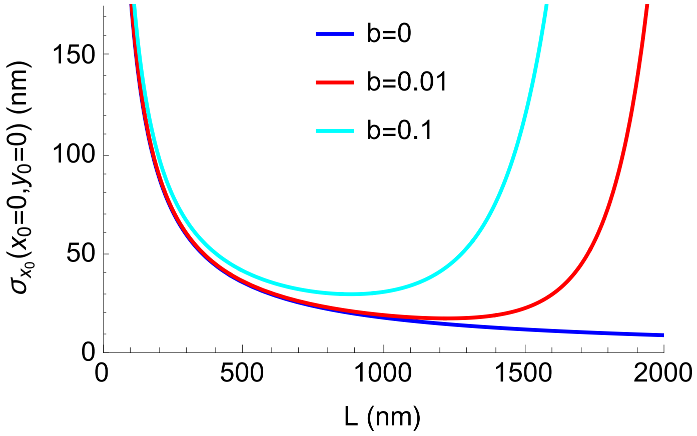


Now let's just point out that we get the same $\sigma_{OT}$ for 4 measurements as for 3.

In[102]:=

```
p0 = f[ang2x[0, R], ang2y[0, R], σq]; p1 = f[ang2x[π / 2, R], ang2y[π / 2, R], σq];
p2 = f[ang2x[π, R], ang2y[π, R], σq];
p3 = f[ang2x[3 π / 2, R], ang2y[3 π / 2, R], σq]; psum = p0 + p1 + p2 + p3;
p0n = p0 / psum; p1n = p1 / psum; p2n = p2 / psum; p3n = p3 / psum;
p0mat =
  {{D[p0n, x0] ^2, D[p0n, x0] * D[p0n, y0]}, {D[p0n, y0] * D[p0n, x0], D[p0n, y0] ^2}};
p1mat =
  {{D[p1n, x0] ^2, D[p1n, x0] * D[p1n, y0]}, {D[p1n, y0] * D[p1n, x0], D[p1n, y0] ^2}};
p2mat =
  {{D[p2n, x0] ^2, D[p2n, x0] * D[p2n, y0]}, {D[p2n, y0] * D[p2n, x0], D[p2n, y0] ^2}};
p3mat =
  {{D[p3n, x0] ^2, D[p3n, x0] * D[p3n, y0]}, {D[p3n, y0] * D[p3n, x0], D[p3n, y0] ^2}};
J = N * ((1 / p0n) * p0mat + (1 / p1n) * p1mat + (1 / p2n) * p2mat + (1 / p3n) * p3mat);
invJ = Inverse[J];
σOT4 = Sqrt[Tr[invJ] / 2];
```

In[111]:=

```
σOT4x0 = FullSimplify[σOT4 /. x0 → 0 /. y0 → 0, {σq > 0, N > 0, L > 0, b > 0}]
```

Out[111]=

$$\frac{2\sqrt{2}\left(1+b\,e^{\frac{L^2}{8\sigma_q^2}}\right)\sigma_q^2}{L\sqrt{N}}$$

In[112]:=

```
FullSimplify[σOT4x0 - σOTx0]
```

Out[112]=

0

Now let's just point out that we get the same $\sigma_{OT}$ for 6 measurements as for 3.

In[113]:=

```
p0 = f[ang2x[0, R], ang2y[0, R], σq]; p1 = f[ang2x[π / 3, R], ang2y[π / 3, R], σq];
p2 = f[ang2x[2 π / 3, R], ang2y[2 π / 3, R], σq]; p3 = f[ang2x[π, R], ang2y[π, R], σq];
p4 = f[ang2x[4 π / 3, R], ang2y[4 π / 3, R], σq];
p5 = f[ang2x[5 π / 3, R], ang2y[5 π / 3, R], σq]; psum = p0 + p1 + p2 + p3 + p4 + p5;
p0n = p0 / psum; p1n = p1 / psum;
p2n = p2 / psum;
p3n = p3 / psum;
p4n = p4 / psum;
p5n = p5 / psum;
p0mat =
  {{D[p0n, x0] ^2, D[p0n, x0] * D[p0n, y0]}, {D[p0n, y0] * D[p0n, x0], D[p0n, y0] ^2}};
p1mat =
  {{D[p1n, x0] ^2, D[p1n, x0] * D[p1n, y0]}, {D[p1n, y0] * D[p1n, x0], D[p1n, y0] ^2}};
p2mat =
  {{D[p2n, x0] ^2, D[p2n, x0] * D[p2n, y0]}, {D[p2n, y0] * D[p2n, x0], D[p2n, y0] ^2}};
p3mat =
  {{D[p3n, x0] ^2, D[p3n, x0] * D[p3n, y0]}, {D[p3n, y0] * D[p3n, x0], D[p3n, y0] ^2}};
p4mat =
  {{D[p4n, x0] ^2, D[p4n, x0] * D[p4n, y0]}, {D[p4n, y0] * D[p4n, x0], D[p4n, y0] ^2}};
p5mat =
  {{D[p5n, x0] ^2, D[p5n, x0] * D[p5n, y0]}, {D[p5n, y0] * D[p5n, x0], D[p5n, y0] ^2}};
J = N * ((1 / p0n) * p0mat + (1 / p1n) * p1mat +
     (1 / p2n) * p2mat + (1 / p3n) * p3mat + (1 / p4n) * p4mat + (1 / p5n) * p5mat);
invJ = Inverse[J];
σOT6 = Sqrt[Tr[invJ] / 2];
```

In[124]:=

```
σOT6x0 = FullSimplify[σOT6 /. x0 → 0 /. y0 → 0, {σq > 0, N > 0, L > 0, b > 0}]
```

Out[124]=

$$\frac{2\sqrt{2}\left(1 + b\, e^{\frac{L^2}{8\sigma_q^2}}\right)\sigma_q^2}{L\sqrt{N}}$$

In[125]:=

```
FullSimplify[σOT6x0 - σOTx0]
```

Out[125]=

0

Now let’s just point out that we get the same $\sigma_{OT}$ for 12 measurements as for 3.

In[126]:=

```
p0 = f[ang2x[0, R], ang2y[0, R], σq]; p1 = f[ang2x[π / 6, R], ang2y[π / 6, R], σq];
p2 = f[ang2x[π / 3, R], ang2y[π / 3, R], σq]; p3 = f[ang2x[π / 2, R], ang2y[π / 2, R], σq];
p4 = f[ang2x[2 π / 3, R], ang2y[2 π / 3, R], σq];
p5 = f[ang2x[5 π / 6, R], ang2y[5 π / 6, R], σq];
```

```
p6 = f[ang2x[π, R], ang2y[π, R], σq];
p7 = f[ang2x[7 π / 6, R], ang2y[7 π / 6, R], σq];
p8 = f[ang2x[4 π / 3, R], ang2y[4 π / 3, R], σq];
p9 = f[ang2x[3 π / 2, R], ang2y[3 π / 2, R], σq];
p10 = f[ang2x[5 π / 3, R], ang2y[5 π / 3, R], σq];
p11 = f[ang2x[11 π / 6, R], ang2y[11 π / 6, R], σq];
psum = p0 + p1 + p2 + p3 + p4 + p5 + p6 + p7 + p8 + p9 + p10 + p11;
p0n = p0 / psum; p1n = p1 / psum;
p2n = p2 / psum;
p3n = p3 / psum;
p4n = p4 / psum;
p5n = p5 / psum; p6n = p6 / psum;
p7n = p7 / psum;
p8n = p8 / psum;
p9n = p9 / psum;
p10n = p10 / psum;
p11n = p11 / psum;
p0mat =
  {{D[p0n, x0] ^2, D[p0n, x0] * D[p0n, y0]}, {D[p0n, y0] * D[p0n, x0], D[p0n, y0] ^2}};
p1mat =
  {{D[p1n, x0] ^2, D[p1n, x0] * D[p1n, y0]}, {D[p1n, y0] * D[p1n, x0], D[p1n, y0] ^2}};
p2mat =
  {{D[p2n, x0] ^2, D[p2n, x0] * D[p2n, y0]}, {D[p2n, y0] * D[p2n, x0], D[p2n, y0] ^2}};
p3mat =
  {{D[p3n, x0] ^2, D[p3n, x0] * D[p3n, y0]}, {D[p3n, y0] * D[p3n, x0], D[p3n, y0] ^2}};
p4mat =
  {{D[p4n, x0] ^2, D[p4n, x0] * D[p4n, y0]}, {D[p4n, y0] * D[p4n, x0], D[p4n, y0] ^2}};
p5mat =
  {{D[p5n, x0] ^2, D[p5n, x0] * D[p5n, y0]}, {D[p5n, y0] * D[p5n, x0], D[p5n, y0] ^2}};
p6mat =
  {{D[p6n, x0] ^2, D[p6n, x0] * D[p6n, y0]}, {D[p6n, y0] * D[p6n, x0], D[p6n, y0] ^2}};
p7mat =
  {{D[p7n, x0] ^2, D[p7n, x0] * D[p7n, y0]}, {D[p7n, y0] * D[p7n, x0], D[p7n, y0] ^2}};
p8mat =
  {{D[p8n, x0] ^2, D[p8n, x0] * D[p8n, y0]}, {D[p8n, y0] * D[p8n, x0], D[p8n, y0] ^2}};
p9mat =
  {{D[p9n, x0] ^2, D[p9n, x0] * D[p9n, y0]}, {D[p9n, y0] * D[p9n, x0], D[p9n, y0] ^2}};
p10mat = {{D[p10n, x0] ^2, D[p10n, x0] * D[p10n, y0]},
   {D[p10n, y0] * D[p10n, x0], D[p10n, y0] ^2}};
p11mat = {{D[p11n, x0] ^2, D[p11n, x0] * D[p11n, y0]},
  {D[p11n, y0] * D[p11n, x0], D[p11n, y0] ^2}};
J = N * ((1 / p0n) * p0mat + (1 / p1n) * p1mat + (1 / p2n) * p2mat + (1 / p3n) * p3mat +
     (1 / p4n) * p4mat + (1 / p5n) * p5mat + (1 / p6n) * p6mat + (1 / p7n) * p7mat +
```

```
    (1 / p8n) * p8mat + (1 / p9n) * p9mat + (1 / p10n) * p10mat + (1 / p11n) * p11mat);
invJ = Inverse[J];
σOT12 = Sqrt[Tr[invJ] / 2];
```

In[142]:=

```
σOT12x0 = FullSimplify[σOT12 /. x0 → 0 /. y0 → 0, {σq > 0, N > 0, L > 0, b > 0}]
```

Out[142]=

$$\frac{2\sqrt{2}\left(1+b\,e^{\frac{L^2}{8\sigma_q^2}}\right)\sigma_q^2}{L\sqrt{N}}$$

In[143]:=

```
FullSimplify[σOT12x0 - σOTx0]
```

Out[143]=

0
